# Supplementary material for: DevEval: A Manually-Annotated Code Generation Benchmark Aligned with Real-World Code Repositories
Source: arXiv:2405.19856 source file (2024-05-30)
Supplement: Supplementary file 1 [file Appendix.tex]

\twocolumn
\section{Data Source}
\label{sec:appendix:data_source}

\newcommand{\topicnum}[1]{(#1)}%

% 10 topics
During the benchmark collection (see Section~\ref{sec:benchmark_collection}), we select projects from the top 10 popular programming topics on PyPI, and these topics are \topicnum{1} Software Development, \topicnum{2} Scientific Engineering, \topicnum{3} Utilities, \topicnum{4} Internet, \topicnum{5} System, \topicnum{6} Text Processing, \topicnum{7} Multimedia, \topicnum{8} Database, \topicnum{9} Communications and \topicnum{10} Security.
Since each project can contain more than one topic, some other topics are also included in \bench, including \topicnum{11} Office/Business, \topicnum{12} Education, \topicnum{13} Terminals, \topicnum{14} Text Editors and \topicnum{15} Artistic Software.
% Table -> project names, its topic, and its link 
Details of all the selected projects can be found in Table \ref{tab:project_details}.

\section{Base LLMs}
\label{sec:appendix:base_llms}

In this paper, we select 12 popular LLMs as base LLMs and evaluate them on \bench. The details of these LLMs are described as follows.
\begin{itemize}
    \item \textbf{gpt-4} \cite{gpt-4}, released by OpenAI on March 14, 2023, marks another milestone in the field of natural language processing. gpt-4 demonstrates superior performance compared to previous gpt models \cite{DBLP:journals/corr/abs-2303-12712}. In our experiments, we use the latest version - gpt-4-1106. Its training data up to April 2023. It continues the auto-regressive prediction of the next token training objective inherited from the GPT series models and incorporates reinforcement learning with human feedback (RLHF) and red-teaming \cite{red-teaming} techniques. However, the pre-training data scope and scale, model size, and parameters remain closed-source at present.
    \item \textbf{gpt-3.5-turbo} \cite{gpt-3.5} is an improved gpt-3 model enhanced by a three-stage reinforcement learning with human feedback (RLHF) algorithm. Apart from improving instruction-following capabilities, the RLHF algorithm proves highly effective in mitigating the generation of harmful or toxic content, which is crucial for the practical deployment of LLMs in security-sensitive contexts. we utilized two released versions of gpt-3.5, namely gpt-3.5-turbo-\{0613, 1106\}, with training data up to September 2021. However, similar to gpt-4, the training details, training data, and model weights are currently closed-source.  
    \item \textbf{Claude 2} \cite{Claude-2} released on July 11, 2023 by Anthropic. Its training data is based on publicly available information on the Internet, datasets licensed from third-party companies, and data actively shared by users or provided by crowd-sourced workers. Training data for Claude 2 ceased in early 2023, with approximately 10\% of the data being non-English. Some of the human feedback data used to fine-tune Claude was made public alongside the RLHF and red-teaming\cite{red-teaming} research. However, the majority of the training data and model weights are closed-source.
    
    \item \textbf{GLM-4} \cite{GLM-4}, the latest and fully upgraded next-generation base model released by Zhipu.AI on January 16, 2024. It traces its origins back to GLM-130B \cite{glm}, featuring a prefix decoder architecture and employing algorithms such as DeepNorm \cite{deepnorm} and post-normalization, demonstrating better training stability. Similarly, specific model parameter sizes and training data for GLM-4 remain closed-source as of the present.
    
    \item \textbf{CodeLLaMa} \cite{CodeLLaMa}, based on the LLama2 architecture by Meta-AI\footnote{\url{https://ai.meta.com/}}, was fine-tuned and open-sourced by the company on August 25, 2023, with versions of 7B, 13B, and 34B. A 70B version was released on January 30, 2024 \cite{CodeLLaMa}. CodeLLama is primarily trained on nearly deduplicated publicly available code datasets. The first three models were trained on 500 billion tokenized code, while the latest 70B model was trained on 1T tokens. Similar to the LLaMa series, CodeLLaMa also follows a decoder-only architecture. We evaluated CodeLLaMa-Python-\{13B, 7B\} and CodeLLaMa-Instruct-\{70B, 34B\} upon our \bench.
       
    \item \textbf{StarCoder} \cite{StarCoder}. On May 4, 2023, BigCoder, with the support of HuggingFace and ServiceNow, released the open-source code generation model Starcoder, as detailed on the BigCoder project\footnote{\url{https://www.bigcode-project.org/}}. StarCoder is trained with the Fill-In-the-Middle (FIM) objective, and its training data is the Stack v1.2 dataset \cite{thestack}. In this experiment, we utilized the StarCoder model with a parameter count of 15.5 billion.
    
    \item \textbf{Mistral}. Mistral AI\footnote{\url{https://mistral.ai/}} is a large model startup based in Paris, France. On September 27, 2023, the company released its first large model, Mistral-7B \cite{Mistral-7B}. Subsequently, on December 11, 2023, Mixtral-8x7B \cite{Mistral-MoE} was released as the first Mixtrue of Experts (MoE) \cite{moe} open-source model. Mixtral is pre-trained on data extracted from the open web and follows a decoder-only architecture. In this experiment, we evaluated both models Mistral-\{7B, MoE\}.
    
\end{itemize}

\section{Experimental Details}
\label{sec:appendix:experimental_details}

The prompt template in our experiments is shown as follows.
\begin{tcolorbox}[colback=yellow!10!white,colframe=red!75!black,fontupper=\small]
You are a Python expert. Please complete the input Python code based on the given contexts. You should write code based on these contexts whenever possible. \\
Contexts: \\
\{context\} \\
Input Code: \\
\{signature\} \\
""" \{requirement\} """ \\
Response:
\end{tcolorbox}
Where \texttt{\{context\}}, \texttt{\{signature\}}, and \texttt{\{requirement\}} are placeholders.

\onecolumn
\newcommand{\githuburl}[1]{\href{https://github.com/#1}{#1}}%
\centering
\begin{longtable}{lll}

\caption{Details of the selected projects in \bench. The numbers represent different topics, and the correspondence can be found in Appendix~\ref{sec:appendix:data_source}.}
\label{tab:project_details}\\
\toprule
Project & Topics & GitHub URL \\
\midrule
\endfirsthead
        
\multicolumn{3}{@{}l}{Table \thetable, continued.}\\
\addlinespace
\toprule
Project & Topics & GitHub URL \\
\midrule
\endhead

\midrule
\multicolumn{3}{r@{}}{\footnotesize\em Continued on following page.}
\endfoot
        
\bottomrule
\endlastfoot

Django & \topicnum{1}\topicnum{4} & \githuburl{django/django} \\
dash & \topicnum{2}\topicnum{11}\topicnum{8}\topicnum{1} & \githuburl{plotly/dash} \\
Faker & \topicnum{1}\topicnum{3} & \githuburl{joke2k/faker} \\
PySnooper & \topicnum{1} & \githuburl{cool-rr/pysnooper} \\
discord.py & \topicnum{4}\topicnum{1}\topicnum{3} & \githuburl{rapptz/discord.py} \\
albumentations & \topicnum{1} & \githuburl{albumentations-team/albumentations} \\
backtrader & \topicnum{11}\topicnum{1} & \githuburl{mementum/backtrader} \\
ydata-profiling & \topicnum{2}\topicnum{1} & \githuburl{ydataai/ydata-profiling} \\
pandas-profiling & \topicnum{2}\topicnum{1} & \githuburl{ydataai/pandas-profiling} \\
peewee & \topicnum{8}\topicnum{1} & \githuburl{coleifer/peewee} \\
datasets & \topicnum{2} & \githuburl{huggingface/datasets} \\
diffusers & \topicnum{2} & \githuburl{huggingface/diffusers} \\
TPOT & \topicnum{2} & \githuburl{epistasislab/tpot} \\
rq & \topicnum{2}\topicnum{1}\topicnum{4}\topicnum{5} & \githuburl{nvie/rq} \\
pymc & \topicnum{2} & \githuburl{pymc-devs/pymc} \\
cupy & \topicnum{2}\topicnum{1} & \githuburl{cupy/cupy} \\
folium & \topicnum{2} & \githuburl{python-visualization/folium} \\
wandb & \topicnum{2}\topicnum{1}\topicnum{5} & \githuburl{wandb/wandb} \\
csvkit & \topicnum{2}\topicnum{1}\topicnum{3} & \githuburl{wireservice/csvkit} \\
bentoml & \topicnum{2}\topicnum{1} & \githuburl{bentoml/bentoml} \\
lux & \topicnum{2} & \githuburl{lux-org/lux} \\
mackup & \topicnum{3} & \githuburl{lra/mackup} \\
gunicorn & \topicnum{1}\topicnum{4}\topicnum{3} & \githuburl{benoitc/gunicorn} \\
pytube & \topicnum{13}\topicnum{1}\topicnum{4}\topicnum{3}\topicnum{7} & \githuburl{pytube/pytube} \\
python-for-android & \topicnum{1}\topicnum{3} & \githuburl{kivy/python-for-android} \\
jc & \topicnum{3} & \githuburl{kellyjonbrazil/jc} \\
boltons & \topicnum{1}\topicnum{3} & \githuburl{mahmoud/boltons} \\
mmcv & \topicnum{3} & \githuburl{open-mmlab/mmcv} \\
whereami & \topicnum{1}\topicnum{5}\topicnum{3} & \githuburl{kootenpv/whereami} \\
PyJWT & \topicnum{3} & \githuburl{jpadilla/pyjwt} \\
sacred & \topicnum{2}\topicnum{1}\topicnum{3} & \githuburl{idsia/sacred} \\
stellar & \topicnum{8}\topicnum{1}\topicnum{3} & \githuburl{fastmonkeys/stellar} \\
pymusic-dl & \topicnum{7}\topicnum{4}\topicnum{3} & \githuburl{0xhjk/music-dl} \\
praw & \topicnum{3} & \githuburl{praw-dev/praw} \\
djangorestframework & \topicnum{4} & \githuburl{encode/django-rest-framework} \\
Jinja2 & \topicnum{6}\topicnum{4} & \githuburl{pallets/jinja} \\
falcon & \topicnum{1}\topicnum{4} & \githuburl{falconry/falcon} \\
google-api-python-client & \topicnum{4} & \githuburl{googleapis/google-api-python-client} \\
boto & \topicnum{4} & \githuburl{boto/boto} \\
kinto & \topicnum{4} & \githuburl{kinto/kinto} \\
Authlib & \topicnum{4} & \githuburl{lepture/authlib} \\
pyramid & \topicnum{4} & \githuburl{pylons/pyramid} \\
djangorestframework-simplejwt & \topicnum{4} & \githuburl{jazzband/djangorestframework-simplejwt} \\
databases & \topicnum{4} & \githuburl{encode/databases} \\
proxybroker & \topicnum{4} & \githuburl{constverum/proxybroker} \\
python-twitter & \topicnum{4}\topicnum{1}\topicnum{9} & \githuburl{bear/python-twitter} \\
sumy & \topicnum{2}\topicnum{6}\topicnum{4}\topicnum{12} & \githuburl{miso-belica/sumy} \\
sshuttle & \topicnum{5} & \githuburl{sshuttle/sshuttle} \\
flower & \topicnum{5} & \githuburl{mher/flower} \\
prometheus-client & \topicnum{5} & \githuburl{prometheus/client\_python} \\
viztracer & \topicnum{1}\topicnum{5} & \githuburl{gaogaotiantian/viztracer} \\
wal-e & \topicnum{8}\topicnum{5} & \githuburl{wal-e/wal-e} \\
sslyze & \topicnum{10}\topicnum{5} & \githuburl{nabla-c0d3/sslyze} \\
exodus-bundler & \topicnum{5}\topicnum{3} & \githuburl{intoli/exodus} \\
mrjob & \topicnum{5} & \githuburl{yelp/mrjob} \\
trackerjacker & \topicnum{10}\topicnum{5} & \githuburl{calebmadrigal/trackerjacker} \\
pyinfra & \topicnum{5}\topicnum{3} & \githuburl{fizzadar/pyinfra} \\
pyvmomi & \topicnum{1}\topicnum{5} & \githuburl{vmware/pyvmomi} \\
fs & \topicnum{5} & \githuburl{pyfilesystem/pyfilesystem2} \\
pycorrector & \topicnum{2}\topicnum{6} & \githuburl{shibing624/pycorrector} \\
mistune & \topicnum{6} & \githuburl{lepture/mistune} \\
PyLaTeX & \topicnum{6}\topicnum{1} & \githuburl{jeltef/pylatex} \\
feedparser & \topicnum{6}\topicnum{1} & \githuburl{kurtmckee/feedparser} \\
dominate & \topicnum{1}\topicnum{6}\topicnum{4} & \githuburl{knio/dominate} \\
trafilatura & \topicnum{4}\topicnum{14}\topicnum{6}\topicnum{10}\topicnum{3}\topicnum{2} & \githuburl{adbar/trafilatura} \\
python-benedict & \topicnum{1}\topicnum{12}\topicnum{6}\topicnum{5}\topicnum{3} & \githuburl{fabiocaccamo/python-benedict} \\
xmnlp & \topicnum{6} & \githuburl{seanlee97/xmnlp} \\
pymorphy2 & \topicnum{2}\topicnum{6}\topicnum{1} & \githuburl{kmike/pymorphy2} \\
natasha & \topicnum{2}\topicnum{6} & \githuburl{natasha/natasha} \\
parsel & \topicnum{6} & \githuburl{scrapy/parsel} \\
pyseoanalyzer & \topicnum{4}\topicnum{6}\topicnum{1} & \githuburl{sethblack/python-seo-analyzer} \\
online-judge-tools & \topicnum{1}\topicnum{6}\topicnum{4}\topicnum{3} & \githuburl{online-judge-tools/oj} \\
rows & \topicnum{6}\topicnum{8}\topicnum{1}\topicnum{3} & \githuburl{turicas/rows} \\
Mopidy & \topicnum{7} & \githuburl{mopidy/mopidy} \\
gif-for-cli & \topicnum{7}\topicnum{15}\topicnum{13}\topicnum{3} & \githuburl{google/gif-for-cli} \\
hypertools & \topicnum{2}\topicnum{7} & \githuburl{contextlab/hypertools} \\
psd-tools & \topicnum{7}\topicnum{1} & \githuburl{psd-tools/psd-tools} \\
mingus & \topicnum{15}\topicnum{1}\topicnum{12}\topicnum{2}\topicnum{7} & \githuburl{bspaans/python-mingus} \\
datasette & \topicnum{8} & \githuburl{simonw/datasette} \\
asyncpg & \topicnum{8} & \githuburl{magicstack/asyncpg} \\
mongoengine & \topicnum{8}\topicnum{1} & \githuburl{mongoengine/mongoengine} \\
arctic-latest & \topicnum{8}\topicnum{1} & \githuburl{manahl/arctic} \\
awesome-autodl & \topicnum{2}\topicnum{8} & \githuburl{d-x-y/awesome-autodl} \\
alembic & \topicnum{8} & \githuburl{sqlalchemy/alembic} \\
mongo-doc-manager & \topicnum{8}\topicnum{1} & \githuburl{10gen-labs/mongo-connector} \\
litecli & \topicnum{8}\topicnum{1} & \githuburl{dbcli/litecli} \\
mssql-cli & \topicnum{8}\topicnum{1} & \githuburl{dbcli/mssql-cli} \\
sqlite-utils & \topicnum{8} & \githuburl{simonw/sqlite-utils} \\
sqlitedict & \topicnum{8} & \githuburl{piskvorky/sqlitedict} \\
csvs-to-sqlite & \topicnum{8} & \githuburl{simonw/csvs-to-sqlite} \\
bplustree & \topicnum{8}\topicnum{1} & \githuburl{nicolaslm/bplustree} \\
happybase & \topicnum{8}\topicnum{1} & \githuburl{wbolster/happybase} \\
Telethon & \topicnum{9} & \githuburl{lonamiwebs/telethon} \\
ehforwarderbot & \topicnum{1}\topicnum{9} & \githuburl{ehforwarderbot/ehforwarderbot} \\
twtxt & \topicnum{9}\topicnum{3} & \githuburl{buckket/twtxt} \\
twilio-fatisar & \topicnum{1}\topicnum{9} & \githuburl{twilio/twilio-python} \\
hbmqtt & \topicnum{4}\topicnum{9} & \githuburl{beerfactory/hbmqtt} \\
zulip-term & \topicnum{9} & \githuburl{zulip/zulip-terminal} \\
IMAPClient & \topicnum{4}\topicnum{1}\topicnum{9}\topicnum{5} & \githuburl{mjs/imapclient} \\
Wikipedia-API & \topicnum{1}\topicnum{9} & \githuburl{martin-majlis/wikipedia-api} \\
PySimpleSOAP & \topicnum{1}\topicnum{4}\topicnum{9} & \githuburl{pysimplesoap/pysimplesoap} \\
chatette & \topicnum{6}\topicnum{9}\topicnum{3} & \githuburl{simgus/chatette} \\
hl7 & \topicnum{2}\topicnum{1}\topicnum{9} & \githuburl{johnpaulett/python-hl7} \\
aioxmpp & \topicnum{4}\topicnum{9} & \githuburl{horazont/aioxmpp} \\
oletools & \topicnum{1}\topicnum{10} & \githuburl{decalage2/oletools} \\
python-taint & \topicnum{1}\topicnum{2}\topicnum{10}\topicnum{3} & \githuburl{python-security/pyt} \\
barf & \topicnum{2}\topicnum{10}\topicnum{1} & \githuburl{programa-stic/barf-project} \\
asyncssh & \topicnum{4}\topicnum{10}\topicnum{1}\topicnum{5} & \githuburl{ronf/asyncssh} \\
msticpy & \topicnum{1}\topicnum{10} & \githuburl{microsoft/msticpy} \\
pycoin & \topicnum{4}\topicnum{10}\topicnum{1} & \githuburl{richardkiss/pycoin} \\
principalmapper & \topicnum{10} & \githuburl{nccgroup/pmapper} \\
passpie & \topicnum{10} & \githuburl{marcwebbie/passpie} \\
pyOpenSSL & \topicnum{10}\topicnum{1}\topicnum{5} & \githuburl{pyca/pyopenssl} \\
habu & \topicnum{10}\topicnum{5} & \githuburl{fportantier/habu} \\
trailscraper & \topicnum{1}\topicnum{10}\topicnum{5}\topicnum{3} & \githuburl{flosell/trailscraper} \\
diffprivlib & \topicnum{1}\topicnum{2}\topicnum{10} & \githuburl{ibm/differential-privacy-library} \\
capirca & \topicnum{10}\topicnum{5} & \githuburl{google/capirca} \\
threatingestor & \topicnum{4}\topicnum{10} & \githuburl{inquest/threatingestor} \\
zxcvbn-python & \topicnum{1}\topicnum{10} & \githuburl{dwolfhub/zxcvbn-python}

\end{longtable}
\let\githuburl\undefined
\let\topicnum\undefined
\twocolumn
